# Supplementary material for: Ultrafast Exciton Decomposition in Transition Metal Dichalcogenide Heterostructures
Source: arXiv:2308.12463 source file (2023-08-23)
Supplement: Supplementary file 1 [file SI.pdf]

# Supplemental Information: Ultrafast Exciton Decomposition in Transition Metal Dichalcogenide Heterostructures

Tomer Amit[1] and Sivan Refaely-Abramson[1]
[1]Department of Molecular Chemistry and Materials Science, Weizmann Institute of Science, Rehovot 7610001, Israel

## I. BSE-based density matrix formalism for exciton-phonon interactions

We work within the framework of the Liouville-von Neumann equation of motion,

$$\frac{\partial \hat{\rho}}{\partial t} = -\frac{i}{\hbar}\left[\hat{H}, \hat{\rho}\right] \tag{1}$$

We define the systems Hamiltonian as:

$$\hat{H} = \hat{H}_0 + \hat{H}' = \hat{H}_{eh} + \hat{H}_{ph} + \hat{H}_{eh-ph} \tag{2}$$

where the non-interacting part, $\hat{H}_0 = \hat{H}_{eh} + \hat{H}_{ph}$, describes pairs of electrons and holes ($eh$) composing the GW-BSE solutions within the exciton basis set [1] and evaluated from $G_0W_0$ on top of density functional theory (DFT) [2]; and of phonon modes ($ph$) computed from density functional perturbation theory (DFPT) [3]. The interaction part, $\hat{H}'$, is perturbative and evaluated through electron($e$)/hole($h$)-phonon coupling.

We compute the time evolution of a density matrix in this representation, following a formalism suggested by Rossi and co workers [4, 5]. In this scheme, a Lindblad-type equation is applied to compute the density matrix propagation in time [6–8]. The phonon degree of freedom is traced out within a Markovian approximation for the quantum Master equation [9]. Here we extend on these previous studies by specifying the time propagation of the electron-hole pairs composing optical excitations upon phonon scattering from first principles.

The initial state is an optically-excited exciton computed from GW-BSE. Within this many-body basis set, the starting point strongly depends on the excitation and the underlying structure, and can generally include multiple transitions between various electron and hole bands, with varying orbital, spin, and momentum properties. We thus define an initial density matrix that can generally be composed of different electron-hole pairs,

$$\hat{\rho}\,(t=0) = |S\rangle\,\langle S|\,, \tag{3}$$

with

$$|S\rangle = \sum_{ehkQ} A^S_{ehkQ}\,|h,k\rangle\,|e,k+Q\rangle \tag{4}$$

an exciton state, and $|A^S_{ehkQ}|^2$ the probability amplitudes for the participating transitions between holes with crystal momentum $k$ and electrons with crystal momentum $k+Q$. The optical excitation is assumed to acquire zero exciton momentum, thus all the initially occupied pairs on the diagonal of $\hat{\rho}\,(t=0)$ have momentum $Q=0$. However, upon phonon scattering, finite $Q$ states can also become occupied, resulting in the observed ultrafast valley and spin transitions demonstrated in this work.

Within this formalism, the time evolution of the density matrix can be derived through:

$$\begin{aligned}\frac{d\rho_{\alpha_i,\alpha_j}}{dt} =& \frac{1}{2}\sum_{\alpha'\alpha'_i\alpha'_j}[(\delta_{\alpha_i\alpha'} - \rho_{\alpha_i\alpha'})P^{eh}_{\alpha'\alpha_j,\alpha'_i\alpha'_j}\rho_{\alpha'_i\alpha'_j} \\ & - (\delta_{\alpha'\alpha'_i} - \rho_{\alpha'_i\alpha'})P^{eh}_{\alpha'\alpha'_i,\alpha_i\alpha'_j}\rho_{\alpha'_j\alpha_j}] + \text{H.c.}\end{aligned} \tag{5}$$

with $\alpha$ representing the electron-hole pairs composing a many-body exciton state. Interactions with phonons are computed with the scattering superoperators:

$$P^{eh}_{eh_1eh_2,eh'_1eh'_2} = P^e_{e_1e_2,e'_1e'_2} + P^h_{h_1h_2,h'_1h'_2} \tag{6}$$

$$P^e_{e_1e_2,e'_1e'_2} = \sum_{\pm,\nu} B^{\nu\pm}_{e_1e'_1}B^{\nu\pm*}_{e_2e'_2}\delta_{h_1h'_1}\delta_{h_2h'_2} \tag{7}$$

$$P^{h}_{h_1h_2,h'_1h'_2} = \sum_{\pm,\nu} B^{\nu\pm}_{h_1h'_1} B^{\nu\pm*}_{h_2h'_2} \delta_{e_1e'_1}\delta_{e_2e'_2} \tag{8}$$

where $P^{e/h}$ describe the scattering of electrons/holes composing the pairs $\alpha$, allowing only one of the particles in the pair to scatter while the other remains unchanged. The coupling to phonons is computed through

$$B^{q\nu\pm}_{pp'} = \sqrt{\frac{2\pi(n_{q\nu}) + \frac{1}{2} \pm \frac{1}{2}}{\hbar}} g^{q\nu}_{pp'} D^{q\nu\pm}_{pp'} \tag{9}$$

for $n_{q\nu}$ the Bose-Einstein occupation function for phonons with momentum $q$ and mode $\nu$, $p = e/h$ for interacting electrons/holes and $g_pp'$ is the particle-phonon coupling. The energy conservation function is

$$D^{q\nu\pm}_{pp'} = \lim_{\sigma\to 0} \frac{\exp(-((\epsilon_{\mathrm{p}} - \epsilon_{\mathrm{p'}} \pm \hbar\omega_{\mathrm{q}\nu})/2\sigma)^2}{(2\pi\sigma^2)^{\frac{1}{4}})} \tag{10}$$

where $\omega_{q\nu}$ the phonon frequency. We note that electron-hole coupling through phonons are neglected in this representation due to the large energy difference between occupied and empty bands composing the excitons, compared to phonon energies ($E_g >> \hbar\omega_{q\nu}$) in the examined systems, even when the electron-hole binding energy is included.

The results obtained from the full density matrix propagation defined in Eq.SI5 are practically equivalent in our case to the result of propagating only the diagonal of the density matrix ($f$):

$$\rho_{\alpha_1,\alpha_2} = f_{\alpha_1}\delta_{\alpha_1,\alpha_2} \tag{11}$$

$$\frac{\partial f_\alpha}{\partial t} = \sum_{\alpha\prime} \left[(1 - f_\alpha)\, P_{\alpha\alpha\prime} f_{\alpha\prime} - (1 - f_{\alpha}\prime)\, P_{\alpha\prime\alpha} f_\alpha\right] \tag{12}$$

with electron/hole-phonon scattering rates:

$$P_{\alpha\alpha\prime} = P_{\alpha\alpha,\alpha\prime\alpha\prime} = |B_{\alpha\alpha\prime}|^2 \tag{13}$$

with $B_{\alpha\alpha\prime}$ defined in Eq.SI9. Thus, the results presented in the main text are achieved with the diagonal propagation, allowing inclusion of more k-points in the propagation.

## II. Computational details

Exciton states and the optical absorption spectrum are calculated within many-body perturbation theory within the GW-BSE approximation [1]. First, the atomic structure, electronic wavefunctions and electronic bandstructure are evaluated from DFT [10] with the Perdew-Burke-Ernzerhof (PBE) exchange-correlation functional [11]. Atomic structure is optimized with the Tkatchenko-Scheffler dispersion corrections [12], leading to an interlayer distance of 6.7Å between metal atoms. We use a Bloch plane-wave basis-set, with norm-conserving pseudopotentials [13] within the Quantum Espresso package [14], including spin-orbit coupling and spinor wavefunctions.

We employ a $30 \times 30 \times 1$ uniform k-grid to compute the self-consistent electron density with a 90 Ry wavefunction cutoff energy. The quasiparticle bandstructure and optical properties are computed within the GW-BSE approximation using the BerkeleyGW software [15]. Quasiparticle energy corrections are calculated within $G_0W_0$ and the generalized plasmon-pole approximation [2], on a uniform $6 \times 6 \times 1$ k-point grid and with 5998 spinor bands and 25 Ry cutoff of the screening function. We then expand our sampling through the Nonuniform Neck Subsampling (NNS) scheme [16] to capture the behavior of the electron wavefunctions accurately throughout the Brillouin zone.

Optical properties are computed by solving the Bethe-Salpeter equation (BSE) [1, 17]. The electron-hole interaction kernel is evaluated including 8 valence and 8 conduction bands and with a dielectric matrix calculated using 1598 bands on a $24 \times 24 \times 1$ k-point grid with a 5 Ry screening cutoff. Exciton wavefunctions and exciton energies are evaluated by interpolation of the interaction kernel onto a $72 \times 72 \times 1$ grid, with linear in-plane light polarization. This grid leads to convergence of the exciton energies within 20 meV. Additional variations in the computed exciton energies occur upon variation of the initial atomic structure; this defines the computational error of the presented exciton energies to be 100 meV.

The calculated absorption spectrum is shown in Fig. S1 (A), with black lines showing the initially-bright states with computed OS> 1 $e^2a_0^2$. The various electron-hole transitions contributing to the initially-bright excitonic states,

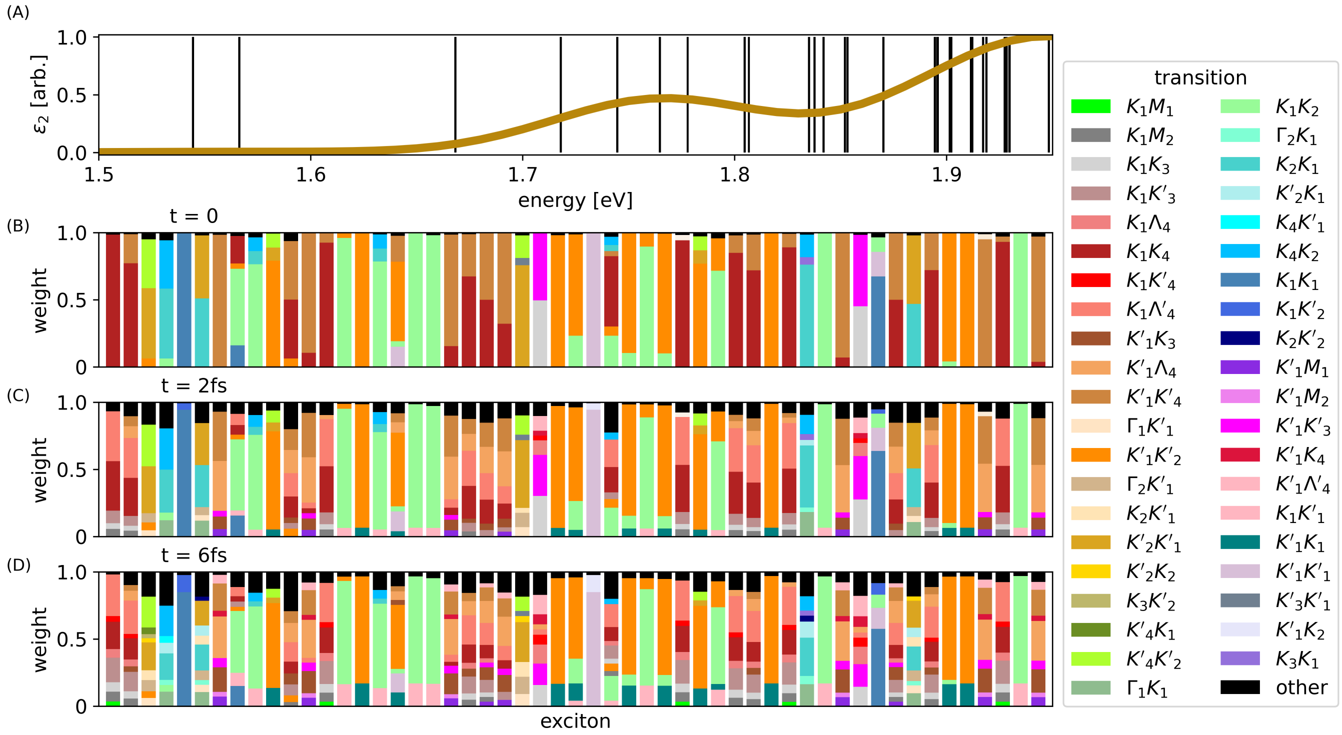


FIG. S1. (A) Computed GW-BSE absorption spectrum for an in-plane light dipole polarization (brown). The black vertical lines mark the energies of the examined excitons. Panels (B,C,D) show the time evolution of the exciton state mixing. Each color represents a different electron-hole transition composing the many-body excitonic state. Each bar corresponds to an initially-bright exciton which is a solution of the BSE, shown for the optical BSE states (B), as well as after 2fs (C) and after 6fs (D) of the propagation.

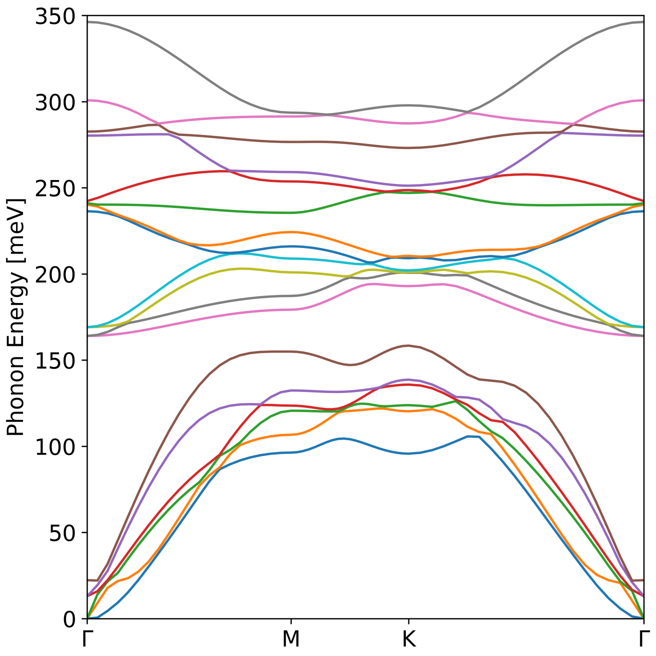


FIG. S2. Phonon bandstructure of the examined $MoSe_2$-$WSe_2$ heterobilayer.

as well as the propagating states, are shown in Fig. S1 (B,C,D) for the three time steps presented in Fig.2 of the main text.

We compute the phononic bandstructure as well as hole-phonon and electron-phonon coupling matrix elements using density matrix perturbation theory [3] within the Quantum Espresso [14] and the EPW packages [18], on a $6 \times 6 \times 1$ uniform q-grid with a convergence energy threshold of $1e^{-19} Ry$. The phononic bandstructure can be seen in Fig. S2.

The density matrix propagation is calculated on a grid of six high-symmetry points Γ, K, K', Λ, Λ′ and M, including 4 hole bands and 4 electron bands. We consider phonon occupation $n_{q\nu}$ at room temperature. The Gaussian broadening of the energy conservation function is $\sigma = 40$ meV. We find an error bar of $\sim 6\%$ induced by varying this broadening in 20 meV. We use a numerical time-step of 0.1 attoseconds.


[1] M. Rohlfing and S. G. Louie, Phys. Rev. Lett. **81**, 2312 (1998).
[2] M. S. Hybertsen and S. G. Louie, Phys. Rev. B **34**, 5390 (1986).
[3] F. Giustino, Rev. Mod. Phys. **89**, 015003 (2017).
[4] R. Rosati, R. C. Iotti, F. Dolcini, and F. Rossi, Phys. Rev. B **90**, 125140 (2014).
[5] R. Rosati, F. Dolcini, and F. Rossi, Phys. Rev. B **92**, 235423 (2015).
[6] D. Manzano, AIP Adv. **10**, 025106 (2020).
[7] F. Rossi, *Theory of semiconductor quantum devices: microscopic modeling and simulation strategies* (Springer Science & Business Media, 2011).
[8] J. Xu, A. Habib, S. Kumar, F. Wu, R. Sundararaman, and Y. Ping, Nat. Commun. **11**, 1 (2020).
[9] R. C. Iotti and F. Rossi, Entropy **22**, 489 (2020).
[10] W. Kohn and L. J. Sham, Phys. Rev. **140**, A1133 (1965).
[11] J. P. Perdew, K. Burke, and M. Ernzerhof, Phys. Rev. Lett. **77**, 3865 (1996).
[12] A. Tkatchenko and M. Scheffler, Phys. Rev. Lett. **102**, 073005 (2009).
[13] M. J. van Setten, M. Giantomassi, E. Bousquet, M. J. Verstraete, D. R. Hamann, X. Gonze, and G.-M. Rignanese, Comput. Phys. Commun. **226**, 39 (2018).
[14] P. Giannozzi, O. Baseggio, P. Bonfà, D. Brunato, R. Car, I. Carnimeo, C. Cavazzoni, S. De Gironcoli, P. Delugas, F. Ferrari Ruffino, *et al.*, J. Chem. Phys. **152** (2020).
[15] J. Deslippe, G. Samsonidze, D. A. Strubbe, M. Jain, M. L. Cohen, and S. G. Louie, Comput. Phys. Commun. **183**, 1269 (2012), 1111.4429.
[16] F. H. da Jornada, D. Y. Qiu, and S. G. Louie, Phys. Rev. B **95**, 035109 (2017), 1610.06641.
[17] M. Rohlfing and S. G. Louie, Phys. Rev. B **62**, 4927 (2000).
[18] S. Poncé, E. R. Margine, C. Verdi, and F. Giustino, Comput. Phys. Commun. **209**, 116 (2016).
